# Supplementary material for: Evaluating Quantized Large Language Models
Source: arXiv:2402.18158 source file (2024-06-06)
Supplement: Supplementary file 1 [file add_related.tex]

\section{Related Work}
\label{app:rw}
